# Supplementary material for: SymphonyQG: Towards Symphonious Integration of Quantization and Graph for Approximate Nearest Neighbor Search
Source: arXiv:2411.12229 source file (2024-11-19)
Supplement: Supplementary file 1 [file edge_supplement.tex]

\begin{algorithm}
\caption{Edge Supplement} \label{alg:edge_supplement}
\begin{algorithmic}[1]

\Require{vertex $v$, maximum out-degree $R$, $v$' out-edges $\mathcal{E}$, $v$'s pruned out-edges $\mathcal{P}$,
        maximum number of iteration $m$}
\Ensure{new set of edges for vertex $v$}

\State{$l \gets 0.5, r \gets 1$}    \Comment{Lower, upper bound of $\cos$}

\If{$|\mathcal{E}| = R$}
    \State \Return{$\mathcal{E}$}
\Else
    \For{$i \gets 1$ to $m$}
        \State{$\mathcal{E}' \gets \mathcal{E}$, $\mathcal{P}' \gets \mathcal{P}$}   
        \State{$t \gets \frac{l+r}{2}$} \Comment{Binary search on cos}
        \While{$\mathcal{P}' \neq \emptyset$}
            \State{$c \gets$ shortest edge in $\mathcal{P}'$}   \Comment{Find candidate}
            \State{Remove $c$ from $\mathcal{P}'$}
            \If{$\forall e \in \mathcal{E}'$, $t \ge$ cos of angle between $e$ and $c$}
                \State{Add $c$ into $\mathcal{E}'$}
            \EndIf
            \If{$|\mathcal{E}'| = R$}
                \State{$\mathbf{break}$}
            \EndIf
        \EndWhile
        \If{$|\mathcal{E}'| = R$}   
            \State{$r \gets t$}
        \Else 
            \State{$l \gets t$}
        \EndIf
    \EndFor
\EndIf
\State{$\mathcal{E}' \gets \mathcal{E}$}
\State{Supplement $\mathcal{E}'$ from $\mathcal{P}$ based on $r$ (same as line 6 to line 14)}.
\State \Return{$\mathcal{E}'$}

\end{algorithmic}
\end{algorithm}
